# Supplementary material for: FiLM: Frequency improved Legendre Memory Model for Long-term Time Series Forecasting
Source: arXiv:2205.08897 source file (2022-09-16)
Supplement: Supplementary file 1 [file mode_selection.tex]

% \section{Mode Selection Policy for FEL}
% \label{app:mode}
% Three different mode selection policies are studied for frequency enhanced layer: 1) lowest mode selection: we select $m$ lowest frequency modes to retain. 2) random model selection: we select $m$ frequency modes randomly to retain. 3) lowest with extra high mode selection: we select $0.8\times m$ lowest frequency modes and $0.2\times m$ high frequency modes randomly to retain. The experimental results are summarized in Table \ref{tab:mode} with $m = 32$ for both experiments.
% \input{tables/tab_mode_selection_policy}
